# Supplementary material for: Dual-Camera Joint Deblurring-Denoising
Source: arXiv:2309.08826 source file (2023-09-16)
Supplement: Supplementary file 1 [file supp_abstract.tex]

Here, we provide the additional material to the main manuscript with the following outline. In Sec.\ \ref{sec:data}, we elaborate on our synthetic data generation pipeline. We discuss details of noise model and blurry data generation that help simulating long and short exposure images. In Sec.\ \ref{sec:results}, we provide more qualitative examples to compare competitive methods, as well as single-task baselines, on both synthetic and real data. Finally, Sec.\ \ref{sec:arch} outlines details of our network architecture.
